# Supplementary material for: Weighted Ensemble Milestoning (WEM): A Combined Approach for Rare Event Simulations
Source: arXiv:1912.10650 ancillary file (2020-07-18)
Supplement: Supplementary file 1 [file supp-info.pdf]

# Supplementary material for: Weighted Ensemble Milestoning (WEM): A Combined Approach for Rare Event Simulations

Dhiman Ray and Ioan Andricioaei

Department of Chemistry, University of California Irvine, California 92697, USA

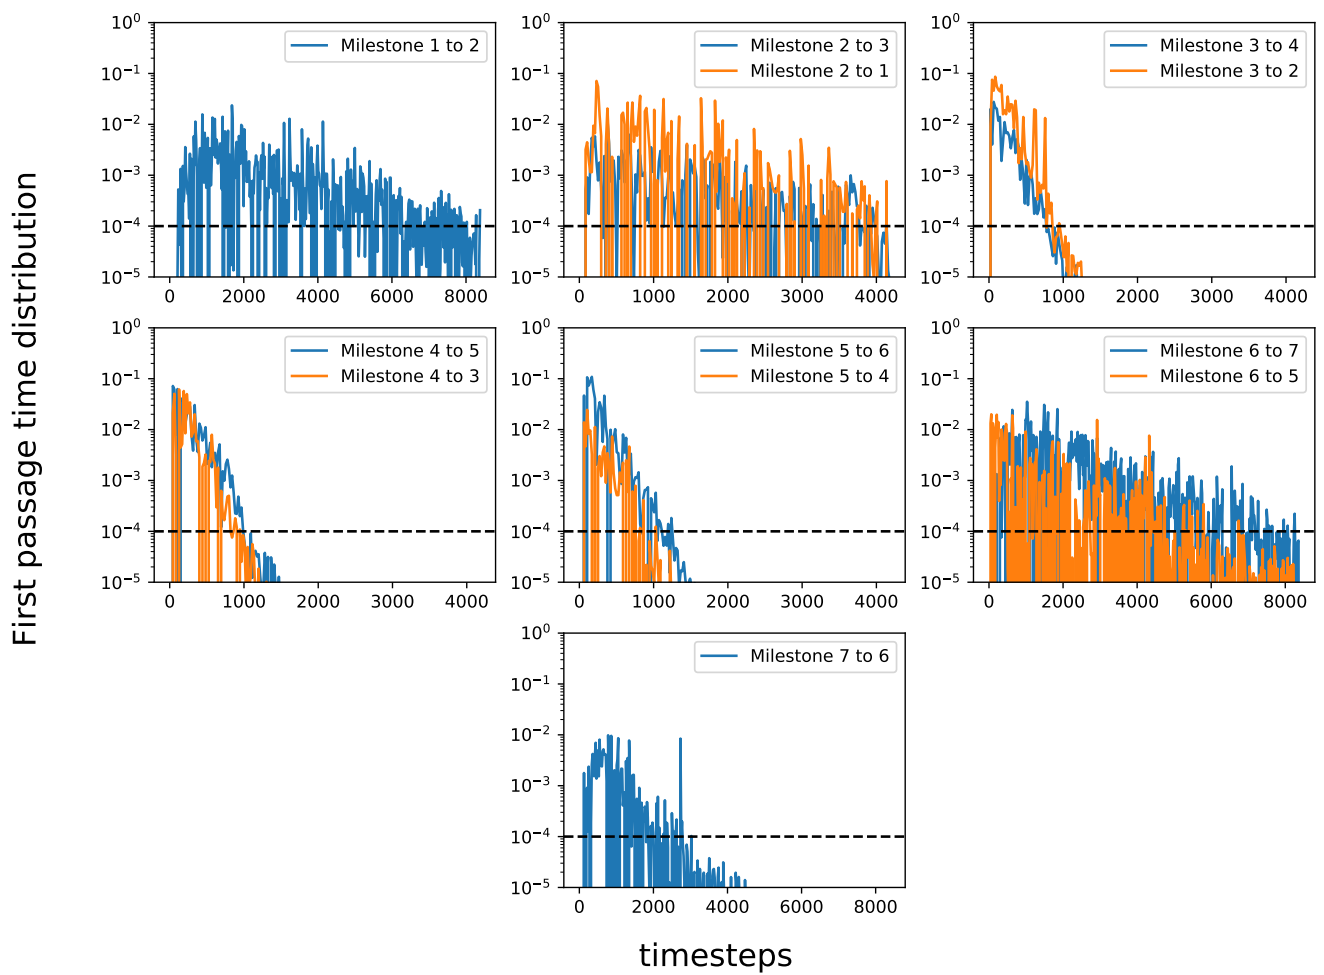

Figure S1: Convergence of first passage time distribution between each pair milestones for (10+1)D coupled potential energy surface (7 milestone case) using WEM method. The results were considered converged when normalized first passage time distribution has fallen below the tolerance of  $10^{-4}$  (marked with dashed horizontal line). The  $x$ -axis is timescale of individual trajectories (molecular timescales) and not total simulation time.

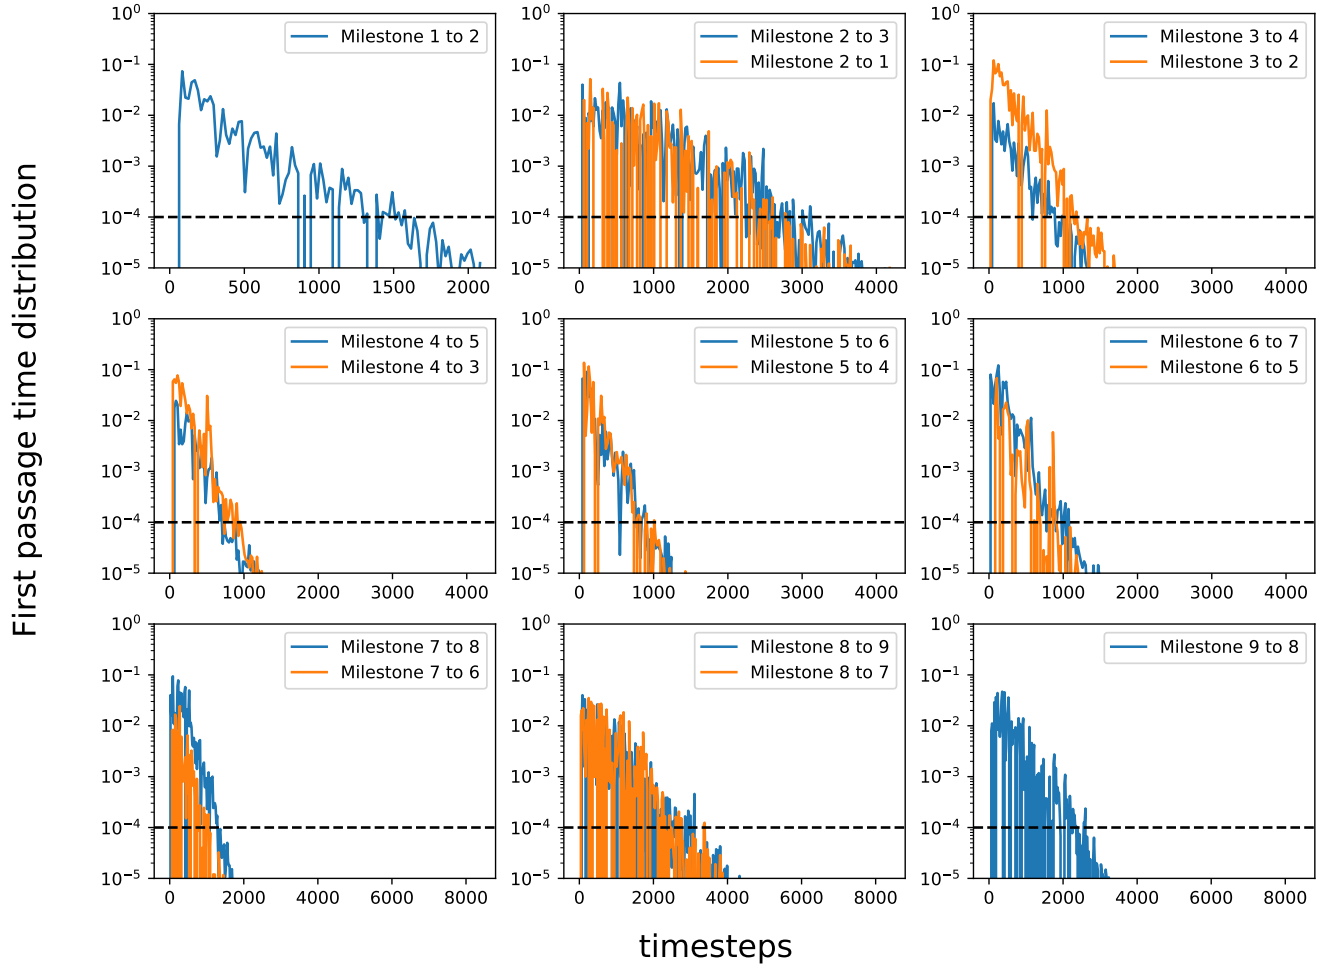

Figure S2: Same as Figure S1 but for 9 milestone case

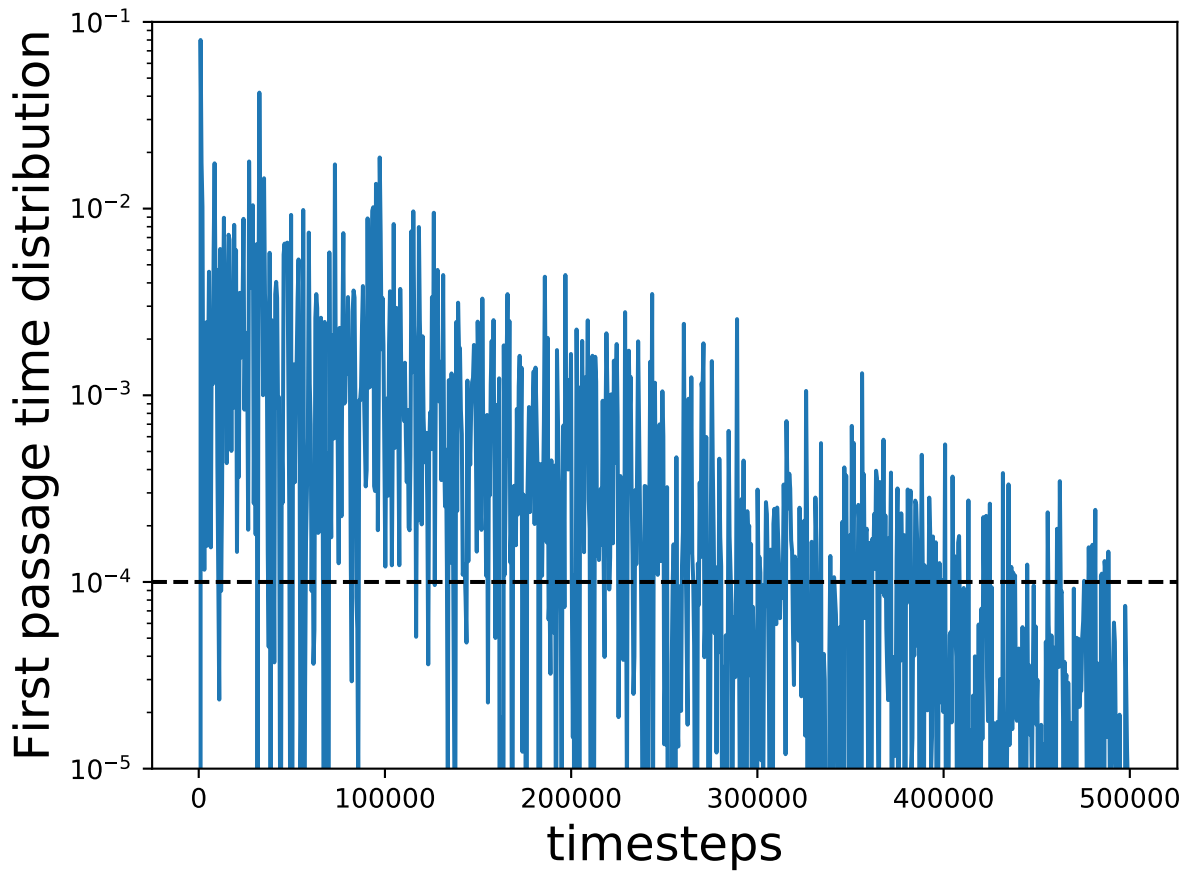

Figure S3: Convergence of mean first passage time for  $x = -1$  to  $x = 1$  transition for (10+1)D coupled potential using conventional equilibrium WE simulation. The  $x$ -axis is timescale of individual trajectories (molecular timescales) and not total simulation time.

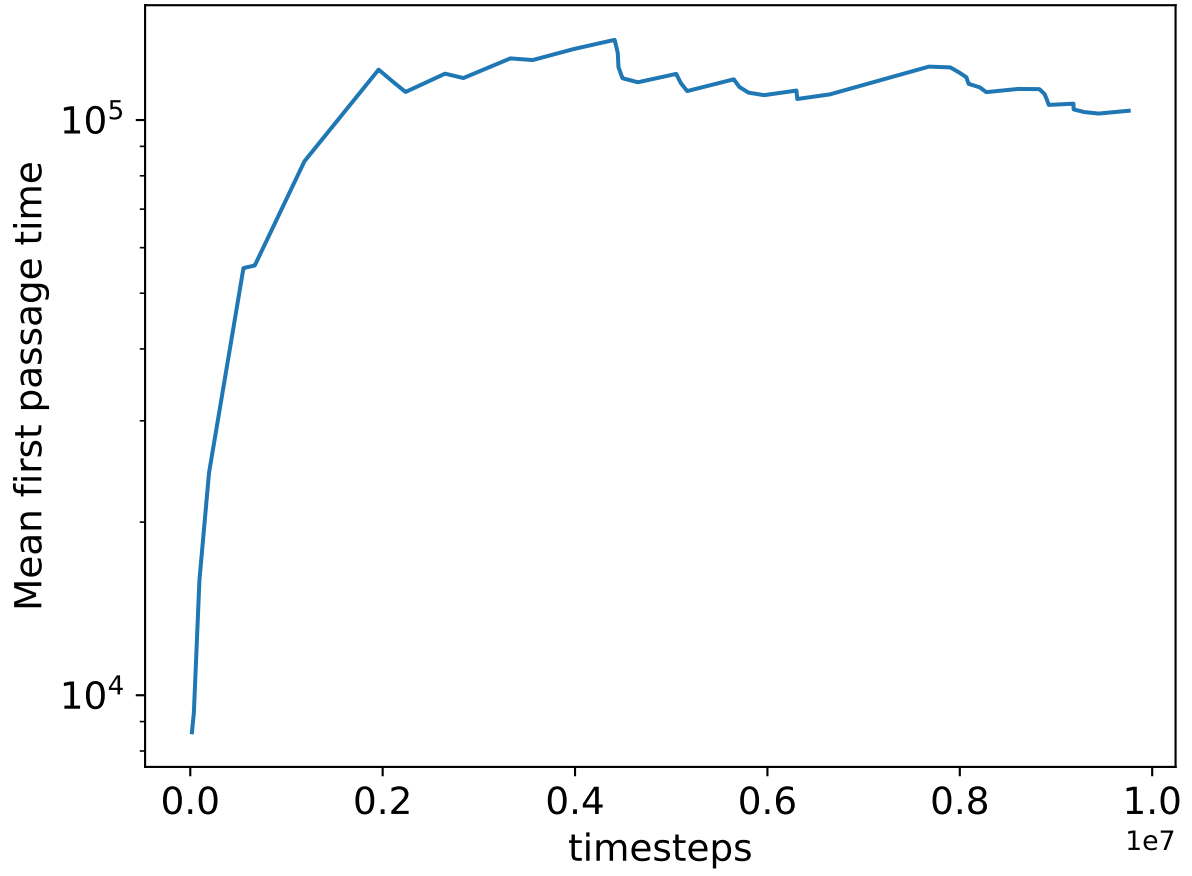

Figure S4: Convergence of mean first passage time for  $x = -1$  to  $x = 1$  transition for (10+1)D coupled potential using regular Langevin Dynamics simulation.

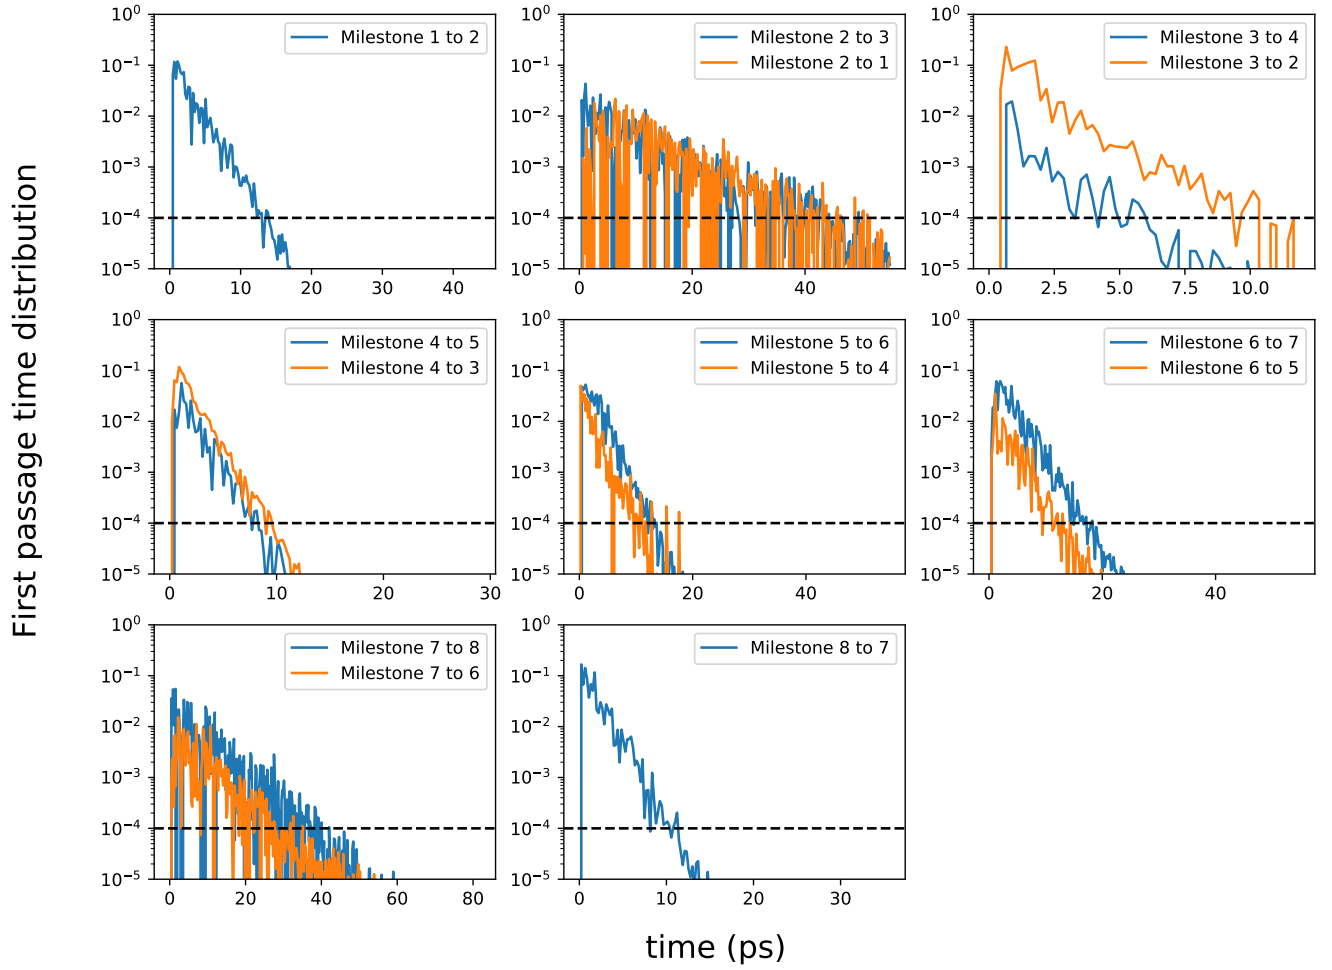

Figure S5: Same as Figure S1 but for Alanine dipeptide  $\alpha_R$  to  $C_{7eq}$  transition with 8 milestones.

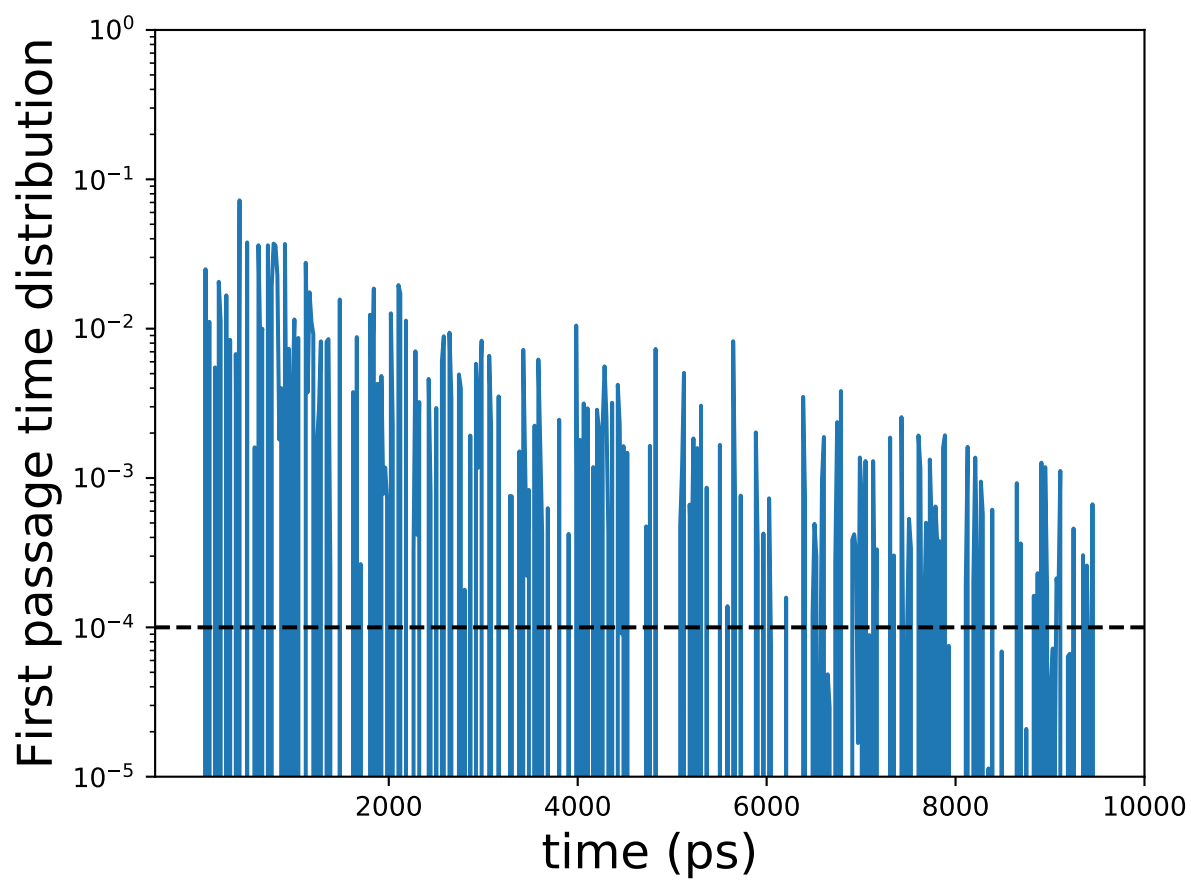

Figure S6: Same as Figure S3 but for Alanine dipeptide  $\alpha_R$  to  $C_{7eq}$  transition

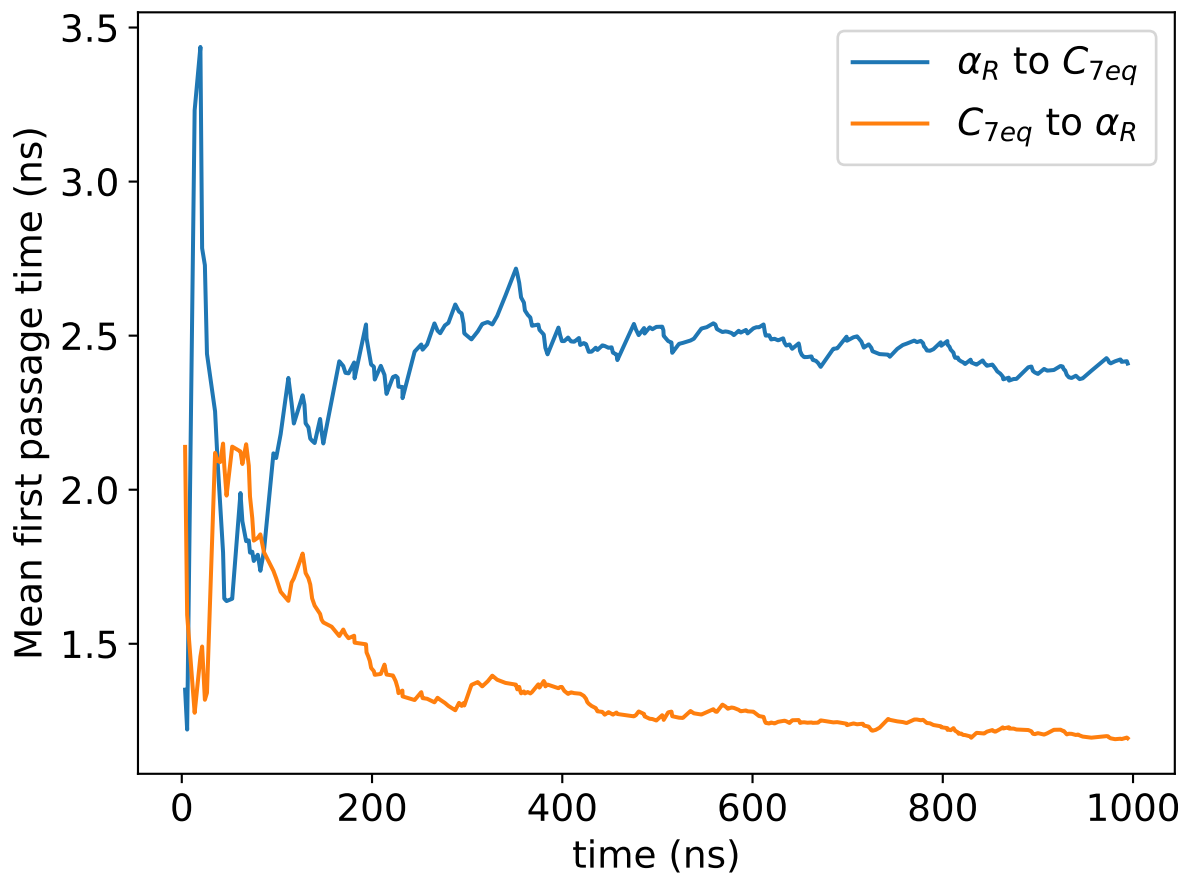

Figure S7: Convergence of Mean first passage time  $\alpha_R$  to  $C_{7eq}$  and the reverse transition in regular MD simulation.
